# Supplementary material for: Long-Term Human Trajectory Prediction using 3D Dynamic Scene Graphs
Source: arXiv:2405.00552 source file (2024-10-30)
Supplement: Supplementary file 1 [file 10_Appendix.tex]

\onecolumn
\newpage
\appendix

\setcounter{figure}{0} 

\twocolumn

\subsection{Human walking at start of trajectory}

We compare the NLL of our method and several baselines on the subset of the dataset where the human is walking at the start of the trajectory rather than interacting with an entity. In this subset, the YNet baseline performs more competitively, however after \SI{3}{s} into the future, the performance of our method surpasses that of both baselines. Note that our method does not directly take the human's walking direction into account.

\begin{figure}[ht!]
    \centering
    \begin{subfigure}{\linewidth}
        \centering
        \includegraphics[width=\linewidth]{figures/nll_office2/nll_stats_walking_start.png}
        \caption{performance in the office environment.}
    \end{subfigure}
    \hfill
    \begin{subfigure}{\linewidth}
        \centering
        \includegraphics[width=\linewidth]{figures/nll_archviz1/nll_stats_walking_start.png}
        \caption{performance in the home environment.}
    \end{subfigure}
    \caption{Negative log-likelihood of our method (blue) and several baselines in both environments on the subset of the dataset where the human is walking at the start of the trajectory rather than interacting with an entity. The shaded background represents one standard deviation.}
    \label{fig:results_nll_walking_start}
\end{figure}

\newpage
\subsection{Upper quartile of distance covered during future trajectory}

We evaluate the NLL of our method and the random walk and random goal na\"\i ve baselines on the subset of the dataset where the traveled distance is above the upper quartile of the dataset. This is to show that in a scenario where the trajectory is less biased towards the startpoint, the random walk baseline performs worse. 

\begin{figure}[ht!]
    \centering
    \begin{subfigure}{\linewidth}
        \centering
        \includegraphics[width=\linewidth]{figures/nll_office2/nll_stats_traveled_distance_future.png}
        \caption{performance in the office environment.}
    \end{subfigure}
    \hfill
    \begin{subfigure}{\linewidth}
        \centering
        \includegraphics[width=\linewidth]{figures/nll_archviz1/nll_stats_traveled_distance_future.png}
        \caption{performance in the home environment.}
    \end{subfigure}
    \caption{Negative log-likelihood of our method (blue) and the random walk na\"\i ve baseline in both environments on the subset of the dataset where the traveled distance is above the upper quartile of the dataset. The shaded background represents one standard deviation. Notice that in this scenario (less biased towards the startpoint), the random walk baseline performs worse.}
    \label{fig:results_nll_distance_upper_quartile}
\end{figure}
